# Supplementary material for: Phase Diagram and Snap-Off Transition for a Twisted Party Balloon
Source: arXiv:2010.08739 source file (2021-01-05)
Supplement: Supplementary file 1 [file Supple_Mat.pdf]

# Supplemental Material: Phase Diagram and Snap-Off Transition for Twisted Balloons

Yu-Chuan Cheng[1], Ting-Heng Hsieh[1], Jih-Chiang Tsai[2], and Tzay-Ming Hong[1,*]
[1]*Department of Physics, National Tsing Hua University, Hsinchu, Taiwan 30013, Republic of China*
[2]*Institute of Physics, Academia Sinica, Taipei, Taiwan 11529, Republic of China*
(Dated: December 25, 2020)

## I. ADDITIONAL DETAILS FOR EXPERIMENTAL SETUP

As shown in Fig. 1(b), the inner diameter of A and B is adjustable. While the weight prevents it from rotating about A, the cylinder B is carefully balanced by a long hollow aluminum pipe of length $S_E$ which in turn is kept stationary by an iron centering pin. The tilt of balloon during twisting is negligible since $s \ll S_E$. In the mean time, the combination of wires of length $W = 5$m and sliding rails that are fixed on the ceiling ensures that the cylinder B moves passively along the central axis as long as the displacement $\Delta z \ll W\sin\alpha$ where $\alpha$ denotes the angle between the wire and ceiling in Fig. 1(b).

## II. BOUNDARY BETWEEN PHASES 1 AND 2

By volume conservation, we obtain the following:

$$\begin{aligned} \pi R^2 L &= \pi R^2 (L^{'} - \ell) + \pi r^2 \ell \\ L^{'} - \ell &= L - \frac{r^2}{R^2}\ell \end{aligned} \tag{S.1}$$

where $L'$ and $\ell$ are defined in Fig. S1(b).

By use of Eq.(S.1), the conserved quantity in Eq.(1) requires that

$$\frac{r^3\theta_1}{\ell} = \frac{R^3(\theta - \theta_1)}{L - \frac{r^2}{R^2}\ell} \tag{S.2}$$

where $\theta_1$ is the portion of shear angle stored in the concaved region. Solving for the $\theta_1$ and subtracting it from $\theta$ give

$$\theta - \theta_1 = \frac{r^3(L - \frac{r^2}{R^2}\ell)\theta}{r^3(L - \frac{r^2}{R^2}\ell)\theta + R^3\ell}. \tag{S.3}$$

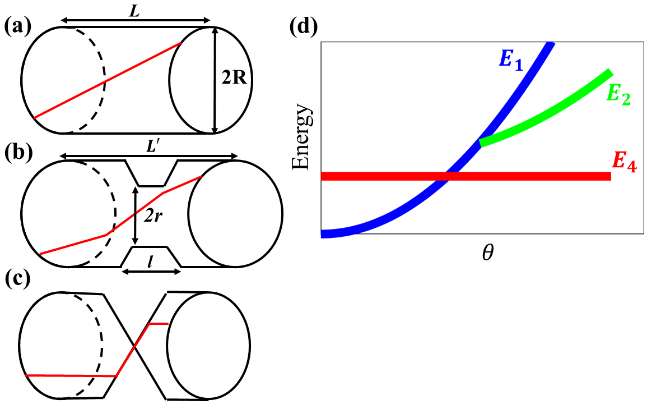


FIG. S1: (a) Simplified model for a twisted balloon where the red line represents the marker we draw on the balloon to help visualize the distribution of shearing angle. (b) Denote the total length of twisted balloon by $L'$, and the diameter and width for the concave segment by $2r$ and $\ell$. (c) Sketch of the snapping phase. Figures (a∼c) are labeled respectively as phase 1, 2 and 4. (d) Schematics for how the potential energy for phase 1, 2, and 4 increases with the twist angle.

Write down the potential energy for phase 2 that consists of shearing and surface tension:

$$E_2 = \frac{SR^3t}{L' - \ell}(\theta - \theta_1)\theta + 2\pi T\Big[R(L' - \ell) + r\ell + (R^2 - r^2) - RL\Big] \tag{S.4}$$

From the relations in Eqs. (S.1, S.3), the above equation can be re-expressed as

$$E_2 = \frac{SR^3t}{L - \frac{r^2}{R^2}\ell}\frac{r^3(L - \frac{r^2}{R^2}\ell)\theta^2}{r^3(L - \frac{r^2}{R^2}\ell) + R^3\ell} + 2\pi T\Big( - \frac{r^2}{R}\ell + r\ell + R^2 - r^2\Big) \tag{S.5}$$

There are two parameters, $\ell$ and $r$, that can used to optimize $E_2$. Minimizing with respect to $\ell$ gives

$$\frac{SR^3tr^3\theta^2}{\Big[r^3(L - \frac{r^2}{R^2}\ell) + R^3\ell\Big]^2}\Big( - \frac{r^5}{R^2} + R^3\Big) = 2\pi T\Big( - \frac{r^2}{R} + r\Big) \tag{S.6}$$

Since we are interested at the critical angle $\theta_{1,2}$ that borders phases 1 and 2, we can set $r = R$ in Eq. (S.6) at the transition:

$$\frac{SR^6t(\theta_{1,2})^2}{R^6L^2}(5R^2) = 2\pi T \tag{S.7}$$

which then gives

$$\theta_{1,2} \sim \sqrt{\frac{T}{St}}\frac{L}{R} \tag{S.8}$$

which is labeled as Eq. (4) in the main text. Now let's tune $r$ to minimize Eq. (S.4). Armed with the knowledge of Eq. (S.8) and $r = R$, the only remaining unknown $\ell$ can be determined as

$$\ell \approx R \tag{S.9}$$

at $\theta_{1,2}$ and is independent of $L$.

## III. MODEL FOR SHRINKING SPEED AT SNAPPING TRANSITION

Since $r$ is much smaller than $R$ at the snapping transition, $r^2\ell/R^2$ term can be neglected compared to $L$ in both the numerator and denominator of Eq. (S.2). Furthermore, the first term $r^3L$ in the denominator can be omitted because $R^3\ell$ is much larger. Based on the above approximations, Eq. (S.2) is simplified to

$$\theta - \theta_1 = \frac{r^3L}{R^3\ell}\theta \tag{S.10}$$

Remember that the distinction between short and medium balloons lies in whether the concave segment spans over the whole balloon. This is based on the result in Eq. (S.9), namely, $\ell \approx R$ at $\theta_{1,2}$. Now imagine cranking up $\theta$ in phase 2. Experimentally both $r$ and $\ell$ are deceased instead of creating another partial segment with aggravated concaveness. This implies that the concave segment can be effectively treated as a down-sized short balloon and $r \sim \ell$ should be valid throughout phases 2 and 3. As a result, we can set $r \sim \ell = \alpha R$ at the snapping transition where $\alpha \ll 1$ decreases with increasing $\theta$. Apparently the twisting direction is arbitrary and so $\alpha$ ought to be an even function of $\theta$ and $\alpha \sim 1/\theta^2$ is the simplest guess:

$$r \sim \ell \sim \frac{R}{(\theta_{3,4})^2} = \frac{SR^2t}{TL} \tag{S.11}$$

at the snapping where the expression for $\theta_{3,4}$ has been borrowed from Eq. (6).

Finally, the shear strain accumulated outside of the concave segment is "sucked" into the bottleneck because $d\theta/dz$ diverges at $r \to 0$ according to Eq. (1). This shear energy is then converted to the kinetic energy of shrinking:

$$\frac{SR^3t}{L}(\theta - \theta_1)^2 \sim \frac{\sigma}{2}\ell rv^2 = \frac{\sigma}{2}(\frac{SR^2t}{TL})^2v^2 \tag{S.12}$$

where $\sigma$ is the surface mass density and Eq. (S.11) has be used. Inputting the formula for $\theta - \theta_1$ in Eq. (S.10) then enables us to determine the shrinking speed as

$$v \sim \Big(\frac{L}{R}\Big)^2\sqrt{\frac{T^3}{S\sigma^2t^2}} \tag{S.13}$$

TABLE I: Comparing properties, with the first four for regime II and the fifth one for III, for selective systems exhibiting the pinch-off where Sh, S, I, V, and D represent shearing, surface tension, inertia, viscosity, and diffusion, and Y/N is the shorthand for yes/no.

| | dominant terms | self-similarity | | memory effect | satellite bubble |
|---|---|---|---|---|---|
| | | $\alpha$ | $\beta$ | | |
| twisting balloon | Sh and I | 2 | 1 | Y | N |
| bubble in capillary tube[a] | S and V | 1 | 1/5 | N | N |
| volume-conserved bubble[b] | S and I | 1 | 1 | N | Y |
| droplet in silicon oil[c] | S and V | 1 | 1 | Y/N | Y |
| ultra-low surface tension[d] | D and V | 1/3 | 1/3 | N | N |
| Bubble in turbulence[e] | S and I | 1/2 | X | N | Y |

[a]Reference [1]
[b]Reference [2]
[c]Reference [3–9]
[d]Reference [10]
[e]Reference [11]

## IV. ANALOGY TO PINCH-OFF PHENOMENON

As is described in the main text, the reason why we checked in Fig. 4(g) and (h) whether the twisted balloon exhibits the self-similarity and lack of memory effect is that these properties are characteristic of the pinch-off phenomenon that looks alike the snap-off transition. But isn't it a long shot to expect a party balloon to behave like a water droplet? In other words, can be analogy be fortuitous? In order to answer this question, it is useful to compile properties, such as the self-similarity, memory effect, and existence of satellite bubble, often associated with pinch-off systems in order to highlight their similarities to and differences from twisted balloons. In addition to the similarities listed in Table I, the snap-off transition is unique in that (1) its scaling exponents $\alpha > \beta$, (2) the retention of memory from the dependence of shrinking velocity on $L/R$, and (3) the surface tension does not enter the behavior of twisted balloons in regime II.

When the viscosity of the interior is much smaller than that of the exterior, as in the case of an air bubble in thick syrup, it has been argued that the system will lose its dependence on the initial conditions. Therefore, scientists often resort to increasing the interior viscosity or decreasing the exterior viscosity in order to retain memory. Balloons provide a new route to achieve that because the viscosity of air is so small that it never enters the equation. Next, how do we know that the shrinking of bottle neck for balloon is not due to the surface energy? The evidence is found experimentally that the titled mark on the straight segment is suddenly straightened when the snap-off occurs. This implies that shearing is the dominant source of energy that is converted to kinetic and competes with the inertia.

---

* ming@phys.nthu.edu.tw

[1] A. A. Pahlavan, H. A. Stone, G. H. McKinley, and R. Juanes, Restoring universality to the pinch-off of a bubble, Proc. Natl. Acad. Sci. U.S.A. **116**, 13780 (2019).
[2] W. C. Li, C. Y. Shih, T. L. Chang, and T. M. Hong (unpublished).
[3] J. Eggers, Universal Pinching of 3D Axisymmetric FreeSurface Flow, Phys. Rev. Lett. **71**, 3458 (1993).
[4] W. W. Zhang and J. R. Lister, Similarity Solutions for Capillary Pinch-Off in Fluids of Differing Viscosity, Phys. Rev. Lett. **83**, 1151 (1999).
[5] X. D. Shi, Michael P. Brenner, and Sidney R. Nagel, A Cascade of Structure in a Drop Falling from a Faucet, Science **265**, 219 (1994).
[6] J. R. Lister and H. A. Stone, Capillary breakup of a viscous thread surrounded by another viscous fluid, Phys. Fluids **10**, 2758 (1998).
[7] I. Cohen, M. P. Brenner, J. Eggers, and S. R. Nagel, Two Fluid Drop Snap-Off Problem: Experiments and Theory, Phys. Rev. Lett. **83**, 1147 (1999).
[8] A. S. Utada, A. Fernandez-Nieves, H. A. Stone, and D. A. Weitz, Dripping to Jetting Transitions in Coflowing Liquid Streams, Phys. Rev. Lett. **99**, 094502 (2007).
[9] M. Rubio, A. Ponce-Torres, E. J. Vega, M. A. Herrada, and J. M. Montanero, Complex behavior very close to the pinching of a liquid free surface, Phys. Rev. Fluids **4**, 021602 (2019).

[10] Hau Yung Lo, Yuan Liu, Sze Yi Mak, Zhuo Xu, Youchuang Chao, Kaye Jiale Li, Ho Cheung Shum, and Lei Xu, Diffusion-Dominated Pinch-Off of Ultralow Surface Tension Fluids, Phys. Rev. Lett. **123**, 134501 (2019)

[11] Daniel J. Ruth, Wouter Mostert, Stphane Perrard, and Luc Deike, Bubble pinch-off in turbulence, Proc. Natl. Acad. Sci. U.S.A. **116**, 25412 (2019).
